# Supplementary material for: Unraveling Consumer Purchase Journey Using Neural Network Models
Source: arXiv:2404.07098 source file (2024-04-10)
Supplement: Supplementary file 1 [file Appendix.tex]

\section{Appendix}\label{sec:appendix}
Table \ref{table:touchpoints} describes the 31 touchpoint types as well as the total counts for each type over the entire 3-year data collection period.

\begin{table}
\begin{tabular}{|c|c|c|c|}
    \hline
    Touchpoint type & Description & Numeric Code & Overall Count \\
    \hline
    Earned social click none & & 1 & 12495\\
    Owned social click none & & 2 & 5167\\
    Paid affiliate click none & & 3 & 2178 \\
    Paid display click awareness & & 4 & 1700\\
    Paid display click nonstock consideration & & 5 & 161\\
    Paid display click nonstock ROI & & 6 & 1287\\
    Paid display click stock consideration & & 7 & 240\\
    Paid display click stock ROI & & 8 & 84\\
    Paid display impression awareness & & 9 & 3278563\\
    Paid display impression nonstock consideration & & 10 & 194759\\
    Paid display impression nonstock ROI & & 11 & 6995656\\
    Paid display impression stock consideration & & 12 & 160837\\
    Paid display impression stock ROI & & 13 & 355639\\
    Paid email click awareness & & 14 & 123190\\
    Paid email click promo & & 15 & 2137\\
    Paid email click ROI & & 16 & 53556\\
    Paid email click stock & & 17 & 8810\\
    Paid email open awareness & & 18 & 1907397\\
    Paid email open promo & & 19 & 65680\\
    Paid email open ROI & & 20 & 814296\\
    Paid email open stock & & 21 & 180003\\
    Paid email sent awareness & & 22 & 2324088\\
    Paid email sent promo & & 23 & 126088\\
    Paid email sent ROI & & 24 & 864342\\
    Paid email sent stock & & 25 & 251481\\
    Paid search click nonstock brand & & 26 & 36123 \\
    Paid search click nonstock nonbrand & & 27 & 11781 \\
    Paid search click stock brand & & 28 & 19139 \\
    Paid search click stock nonbrand & & 29 & 3240 \\
    Paid social click paid FB & & 30 & 78 \\
    Paid social impression paid FB & & 31 & 30402 \\
    \hline
\end{tabular}\caption{Touchpoint descriptions and counts.}
\end{table}\label{table:touchpoints}
